# Supplementary material for: Auto-Configuring Entity Resolution Pipelines
Source: arXiv:2503.13226 source file (2025-03-17)
Supplement: Supplementary file 1 [file 8_appendix.tex]

\section{Appendix}\label{sec:appendix}

\begin{table}[ht]
\centering
\caption{Parameters Tested for RF Regression Method.}
\label{tab:regressor_params}
\begin{tabular}{|p{1.5cm}|l|l|}
\hline
\textbf{Regressor}          & \textbf{Parameter}        & \textbf{Search Space}                           \\ \hline
% \multirow{1}{*}{Lasso}      & alpha                     & \text{LogUniform}($10^{-4}$, $10^1$)                           \\ \hline
% \multirow{1}{*}{Ridge}      & alpha                     & \text{LogUniform}($10^{-4}$, $10^1$)                           \\ \hline
% \multirow{1}{*}{LR} & -                 & -                                               \\ \hline
% \multirow{8}{*}{XGBR} & n\_estimators    & $\{100,...,1000\} \subseteq \mathbb{Z}$                                   \\ \cline{2-3}
%                             & max\_depth                 & $\{3,...,10\} \subseteq \mathbb{Z}$                                      \\ \cline{2-3}
%                             & learning\_rate             & \text{LogUniform}($10^{-3}$, $10^{-1}$)                          \\ \cline{2-3}
%                             & subsample                 & \text{Uniform}($0.5$, $1.0$)                                                \\ \cline{2-3}
%                             & colsample\_bytree          & \text{Uniform}($0.5$, $1.0$)                               \\ \cline{2-3}
%                             & gamma                     & $\{0,...,5\} \subseteq \mathbb{Z}$                                        \\ \cline{2-3}
%                             & reg\_alpha                 & \text{LogUniform}($10^{-2}$, $10^{2}$)                              \\ \cline{2-3}
%                             & reg\_lambda                & \text{LogUniform}($10^{-2}$, $10^{2}$)                              \\ \hline
\multirow{5}{*}{RFR} & n\_estimators & $\{100, ..., 1000\} \subseteq \mathbb{Z}$                                  \\ \cline{2-3}
                            & max\_depth                 &  $\{3,...,10\} \subseteq \mathbb{Z}$                                      \\ \cline{2-3}
                            & min\_samples\_split         &  $\{2,...,20\} \subseteq \mathbb{Z}$                                      \\ \cline{2-3}
                            & min\_samples\_leaf          &  $\{1,...,20\} \subseteq \mathbb{Z}$                                      \\ \cline{2-3}
                            & max\_features              & $\{ sqrt, log2\}$                            \\ \hline
% \multirow{3}{*}{NN}         & hidden\_dim                &  $\{16,...,128\} \subseteq \mathbb{Z}$                                    \\ \cline{2-3}
%                             & lr                         & \text{LogUniform}($10^{-5}, 10^{-2}$)                          \\ \cline{2-3}
%                             & num\_epochs                &  $\{2,...,50\} \subseteq \mathbb{Z}$                                      \\ \hline
\end{tabular}
\end{table}
